# Supplementary material for: A bijection between permutation matrices and descending plane partitions without special parts, which respects the quadruplet of statistics considered by Behrend, Di Francesco and Zinn--Justin
Source: arXiv:1806.05381 source file (2018-09-07)
Supplement: Supplementary file 1 [file appendix.tex]

Idea: DPPs are a folded and twisted ``code'' of ASMs, destroying the ``apparent symmetries''.

It is very easy to see: The numbers of inversions and antiinversions in every \EM{kinked path}
are equal.

By symmetry, it suffices to show this for kinked paths moving right/downwards. Replace every entry
of the \ASM\ to the right or above the kinked path with zero and observe:
\bit
\item the number of inversions plus the number of $1$--s in the path equals the number of columns with column sum $1$,
\item the number of antiinversions plus the number of $1$--s in the path equals the number of 
rows with column sum $1$.
\eit
%Diese Anzahlen müssen also gleich sein. QED.
%
%D.h.: Die $n$ geknickten rechts/unten Pfade eine $n$--ASM bilden eine \EM{Partition} von Inversionen und
%Antiinversionen in Blöcke, die immer gleich viel Inversionen und Antiinversionen enthalten.
